# Supplementary material for: A Conditional Denoising Diffusion Probabilistic Model for Radio Interferometric Image Reconstruction
Source: arXiv:2305.09121 source file (2023-08-29)
Supplement: Supplementary file 1 [file supplement.tex]

supplementary
